# Supplementary material for: Low-scaling $GW$ with benchmark accuracy and application to phosphorene nanosheets
Source: arXiv:2012.06321 ancillary file (2021-03-08)
Supplement: Supplementary file 1 [file supporting_info.pdf]

# Supplemental Material to "Low-scaling *GW* with benchmark accuracy and application to phosphorene nanosheets"

Jan Wilhelm,[1,*] Patrick Seewald,[2] and Dorothea Golze[3]

[1]*Institute of Theoretical Physics, University of Regensburg, D-93053 Regensburg, Germany*
[2]*Department of Chemistry, University of Zurich, CH-8057 Zurich, Switzerland*
[3]*Department of Applied Physics, Aalto University, FI-00076 Aalto, Finland*

(Dated: December 10, 2020)

In this Supporting Information, we show that RI factorizations with a plane-wave RI basis set are independent of the RI metric (Sec. I), we provide all HOMO and LUMO values of the *GW*100 test set (Sec. II), a CP2K input file for a *GW*100 calculation (Sec. III), a basis set convergence test on a small phosphorene nanosheet (Sec. IV), the customized RI basis set for hydrogen and phosphorus (Sec. V) and and an input file for a large-scale phosphorene calculation (Sec. VI).

## I. EQUIVALENCE OF RI METRICS IN A PLANE-WAVE RI BASIS SET

We show in this section, that the RI factorization from the main text in a plane-wave RI basis $\{\mathbf{G}\}$ is identical, irregardless, which metric $m(\mathbf{r},\mathbf{r}') = m(\mathbf{r}-\mathbf{r}')$ is used. We start from the RI factorization

$$(\mu\nu|\lambda\sigma)_{\text{RI}} = \sum_{\mathbf{G}\mathbf{G}'\mathbf{G}''\mathbf{G}'''} (\mu\nu|\mathbf{G})_m M^{-1}_{\mathbf{G}\mathbf{G}'} V_{\mathbf{G}'\mathbf{G}''} M^{-1}_{\mathbf{G}''\mathbf{G}'''} (\mathbf{G}'''|\lambda\sigma)_m\,, \tag{1}$$

where, omitting normalizations, we have for a metric $m(\mathbf{r},\mathbf{r}') = m(\mathbf{r}-\mathbf{r}')$:

$$M_{\mathbf{G}\mathbf{G}'} = \int d\mathbf{r}\,d\mathbf{r}'\,e^{i\mathbf{G}\mathbf{r}} m(\mathbf{r}-\mathbf{r}') e^{-i\mathbf{G}'\mathbf{r}'} \overset{\mathbf{r}=\mathbf{r}'+\mathbf{r}''}{=} \int d\mathbf{r}'\,d\mathbf{r}''\,e^{i\mathbf{G}(\mathbf{r}'+\mathbf{r}'')} m(\mathbf{r}'') e^{-i\mathbf{G}'\mathbf{r}'} = \left(\int d\mathbf{r}\,e^{i(\mathbf{G}-\mathbf{G}')\mathbf{r}}\right)\left(\int d\mathbf{r}\,e^{i\mathbf{G}'\mathbf{r}} m(\mathbf{r})\right) = \delta_{\mathbf{G}\mathbf{G}'}\,m_{\mathbf{G}} \tag{2}$$

with $\delta_{\mathbf{G}\mathbf{G}'}$ being the Kronecker symbol and defining

$$m_{\mathbf{G}} := \int d\mathbf{r}\,e^{i\mathbf{G}\mathbf{r}} m(\mathbf{r})\,, \tag{3}$$

such that

$$M^{-1}_{\mathbf{G}\mathbf{G}'} = \delta_{\mathbf{G}\mathbf{G}'}\,\frac{1}{m_{\mathbf{G}}}\,. \tag{4}$$

Omitting normalizations, the three-center integrals read

$$(\mu\nu|\mathbf{G})_m = \int d\mathbf{r}\,d\mathbf{r}'\varphi_\nu(\mathbf{r})\,\varphi_\mu(\mathbf{r})\,m(\mathbf{r}-\mathbf{r}')\,e^{-i\mathbf{G}\mathbf{r}'} = \left(\int d\mathbf{r}\,\varphi_\nu(\mathbf{r})\,\varphi_\mu(\mathbf{r})\,e^{-i\mathbf{G}\mathbf{r}}\right)\left(\int d\mathbf{r}\,e^{i\mathbf{G}\mathbf{r}} m(\mathbf{r})\right) = (\mu\nu\mathbf{G})\,m_{\mathbf{G}} \tag{5}$$

defining

$$(\mu\nu\mathbf{G}) := \int d\mathbf{r}\,\varphi_\nu(\mathbf{r})\,\varphi_\mu(\mathbf{r})\,e^{-i\mathbf{G}\mathbf{r}}\,. \tag{6}$$

Using $V_{\mathbf{G}\mathbf{G}'} = \delta_{\mathbf{G}\mathbf{G}'}/|\mathbf{G}|^2$ and Eqs. (4), (5), the RI factorization (1) with a plane-wave RI basis reads

$$(\mu\nu|\lambda\sigma)_{\text{RI}} = \sum_{\mathbf{G}} \frac{(\mu\nu\mathbf{G})\,(\mathbf{G}\lambda\sigma)}{|\mathbf{G}|^2}\,. \tag{7}$$

The result (7) is independent of the metric $m$ such that RI factorizations in a plane-wave basis set are identical, irregardless of the metric $m$.

## II. $GW$100 BENCHMARK

TABLE I. $G_0W_0$@PBE HOMO and LUMO energies in eV at the def2-QZVP level for the $GW$100[1] benchmark set. Presented are the values from the cubic-scaling $GW$ algorithm with RI-tC implemented in CP2K and the reference values from FHI-aims reported in Ref. 1. In both cases, analytic continuation with a 16-parameter Padé approximant is used. HOMO values in brackets (BN, BeO, MgO, $O_3$, CuCN) have been excluded from the benchmark since these molecules have been computed with 128 Padé parameters in the FHI-aims reference.

| | HOMO | | LUMO | |
|---|---|---|---|---|
| Molecule | FHI-aims 16-pole[1] | CP2K $O(N^3)$ | FHI-aims 16-pole[1] | CP2K $O(N^3)$ |
| 1 He | -23.48 | -23.48 | 11.00 | 11.01 |
| 2 Ne | -20.37 | -20.38 | 11.64 | 11.64 |
| 3 Ar | -15.12 | -15.13 | 8.10 | 8.11 |
| 4 Kr | -13.54 | -13.57 | 7.63 | 7.63 |
| 5 Xe | -11.99 | -12.02 | 7.93 | 7.98 |
| 6 $H_2$ | -15.80 | -15.81 | 3.50 | 3.50 |
| 7 $Li_2$ | -4.98 | -4.99 | -0.64 | -0.63 |
| 8 $Na_2$ | -4.81 | -4.83 | -0.56 | -0.55 |
| 9 $Na_4$ | -4.11 | -4.10 | -1.02 | -1.01 |
| 10 $Na_6$ | -4.24 | -4.24 | -0.97 | -0.97 |
| 11 $K_2$ | -3.97 | -3.98 | -0.65 | -0.65 |
| 12 $Rb_2$ | -3.79 | -3.80 | -0.63 | -0.62 |
| 13 $N_2$ | -14.90 | -14.89 | 2.45 | 2.45 |
| 14 $P_2$ | -10.21 | -10.21 | -0.72 | -0.72 |
| 15 $As_2$ | -9.47 | -9.47 | -0.85 | -0.85 |
| 16 $F_2$ | -14.95 | -14.96 | -0.71 | -0.70 |
| 17 $Cl_2$ | -11.10 | -11.10 | -0.90 | -0.89 |
| 18 $Br_2$ | -10.22 | -10.22 | -1.39 | -1.40 |
| 19 $I_2$ | -9.28 | -9.28 | -1.69 | -1.68 |
| 20 $CH_4$ | -13.93 | -13.93 | 2.44 | 2.45 |
| 21 $C_2H_6$ | -12.36 | -12.37 | 2.28 | 2.29 |
| 22 $C_3H_8$ | -11.79 | -11.79 | 2.18 | 2.19 |
| 23 $C_4H_{10}$ | -11.48 | -11.49 | 2.13 | 2.14 |
| 24 $C_2H_4$ | -10.32 | -10.33 | 2.02 | 2.02 |
| 25 $C_2H_2$ | -11.02 | -11.02 | 2.86 | 2.86 |
| 26 $C_4$ | -10.78 | -10.78 | -2.93 | -2.94 |
| 27 $C_3H_6$ | -10.55 | -10.56 | 2.44 | 2.45 |
| 28 $C_6H_6$ | -8.98 | -8.99 | 1.08 | 1.09 |
| 29 $C_8H_8$ | -8.05 | -8.06 | 0.06 | 0.06 |
| 30 $C_5H_6$ | -8.35 | -8.35 | 1.04 | 1.04 |
| 31 $C_2H_3F$ | -10.20 | -10.20 | 2.14 | 2.15 |
| 32 $C_2H_3Cl$ | -9.76 | -9.76 | 1.42 | 1.42 |
| 33 $C_2H_3Br$ | -8.99 | -8.99 | 1.38 | 1.38 |
| 34 $C_2H_3I$ | -9.04 | -9.04 | 0.88 | 0.89 |
| 35 $CF_4$ | -15.37 | -15.37 | 4.41 | 4.41 |
| 36 $CCl_4$ | -10.96 | -10.98 | -0.01 | -0.01 |
| 37 $CBr_4$ | -9.89 | -9.90 | -1.08 | -1.08 |
| 38 $CI_4$ | -8.83 | -8.82 | -2.14 | -2.14 |
| 39 $SiH_4$ | -12.30 | -12.31 | 2.50 | 2.51 |
| 40 $GeH_4$ | -12.02 | -12.02 | 2.31 | 2.30 |
| 41 $Si_2H_6$ | -10.30 | -10.31 | 1.68 | 1.69 |
| 42 $Si_5H_{12}$ | -8.93 | -8.94 | 0.16 | 0.16 |
| 43 LiH | -6.55 | -6.54 | -0.08 | -0.07 |
| 44 KH | -4.85 | -4.86 | -0.18 | -0.18 |
| 45 $BH_3$ | -12.87 | -12.87 | 0.12 | 0.12 |
| 46 $B_2H_6$ | -11.83 | -11.84 | 0.84 | 0.84 |
| 47 $NH_3$ | -10.31 | -10.32 | 2.31 | 2.31 |
| 48 $HN_3$ | -10.40 | -10.39 | 1.40 | 1.40 |
| 49 $PH_3$ | -10.26 | -10.27 | 2.49 | 2.50 |
| 50 $AsH_3$ | -10.11 | -10.12 | 2.31 | 2.32 |

TABLE II. Continuation of Table I.

| Molecule | HOMO FHI-aims 16-pole[1] | HOMO CP2K $O(N^3)$ | LUMO FHI-aims 16-pole[1] | LUMO CP2K $O(N^3)$ |
|---|---|---|---|---|
| 51 $SH_2$ | -10.01 | -10.03 | 2.56 | 2.56 |
| 52 HF | -15.30 | -15.30 | 2.54 | 2.54 |
| 53 HCl | -12.24 | -12.25 | 2.05 | 2.06 |
| 54 LiF | -9.93 | -9.95 | 0.09 | 0.09 |
| 55 $MgF_2$ | -12.32 | -12.32 | -0.14 | -0.14 |
| 56 $TiF_4$ | -13.89 | -13.89 | -0.60 | -0.60 |
| 57 $AlF_3$ | -14.25 | -14.25 | 0.16 | 0.16 |
| 58 BF | -10.56 | -10.56 | 1.22 | 1.22 |
| 59 $SF_4$ | -12.11 | -12.12 | 0.38 | 0.38 |
| 60 BrK | -7.28 | -7.30 | -0.32 | -0.31 |
| 61 GaCl | -9.55 | -9.55 | -0.03 | -0.02 |
| 62 NaCl | -8.11 | -8.10 | -0.40 | -0.39 |
| 63 $MgCl_2$ | -10.98 | -10.99 | -0.43 | -0.43 |
| 64 $AlI_3$ | -9.32 | -9.32 | -0.80 | -0.80 |
| 65 BN | -11.23 | (-11.03) | -3.86 | -3.88 |
| 66 NCH | -13.21 | -13.21 | 2.58 | 2.58 |
| 67 PN | -11.13 | -11.14 | -0.20 | -0.20 |
| 68 $N_2H_4$ | -9.27 | -9.28 | 1.99 | 1.99 |
| 69 $H_2CO$ | -10.32 | -10.33 | 0.95 | 0.96 |
| 70 $CH_3OH$ | -10.56 | -10.56 | 2.24 | 2.25 |
| 71 $C_2H_5OH$ | -10.15 | -10.16 | 2.06 | 2.08 |
| 72 $C_2H_4O$ | -9.54 | -9.55 | 1.07 | 1.05 |
| 73 $C_4H_{10}O_4$ | -9.32 | -9.32 | 2.08 | 2.10 |
| 74 HCOOH | -10.73 | -10.73 | 1.91 | 1.91 |
| 75 $H_2O_2$ | -10.98 | -10.99 | 2.34 | 2.35 |
| 76 $H_2O$ | -11.97 | -11.97 | 2.36 | 2.37 |
| 77 $CO_2$ | -13.25 | -13.25 | 2.50 | 2.50 |
| 78 $CS_2$ | -9.75 | -9.75 | -0.20 | -0.20 |
| 79 OCS | -10.91 | -10.91 | 1.21 | 1.21 |
| 80 OCSe | -10.20 | -10.20 | 0.85 | 0.87 |
| 81 CO | -13.57 | -13.57 | 0.68 | 0.67 |
| 82 $O_3$ | -11.62 | (-11.39) | -2.30 | -2.30 |
| 83 $SO_2$ | -11.82 | -11.82 | -1.00 | -1.00 |
| 84 BeO | -8.77 | (-8.58) | -2.49 | -2.49 |
| 85 MgO | -6.75 | (-6.68) | -1.89 | -1.89 |
| 86 $C_7H_8$ | -8.61 | -8.61 | 1.01 | 1.01 |
| 87 $C_8H_{10}$ | -8.55 | -8.55 | 1.04 | 1.04 |
| 88 $C_6F_6$ | -9.49 | -9.49 | 0.65 | 0.66 |
| 89 $C_6H_5OH$ | -8.36 | -8.37 | 0.96 | 0.96 |
| 90 $C_6H_5NH_2$ | -7.64 | -7.64 | 1.14 | 1.15 |
| 91 $C_5H_5N$ | -9.03 | -9.04 | 0.51 | 0.51 |
| 92 guanine | -7.69 | -7.69 | 0.74 | 0.74 |
| 93 adenine | -7.97 | -7.98 | 0.47 | 0.47 |
| 94 cytosin | -8.28 | -8.29 | 0.26 | 0.26 |
| 95 thymine | -8.70 | -8.71 | 0.06 | 0.06 |
| 96 uracil | -9.22 | -9.22 | 0.01 | 0.01 |
| 97 urea | -9.32 | -9.32 | 1.62 | 1.62 |
| 98 $Ag_2$ | -7.07 | -7.07 | -0.89 [a] | -0.89 |
| 99 $Cu_2$ | -7.60 | -7.55 | -0.93 | -0.92 |
| 100 CuCN | -9.72 | (-9.42) | -1.68 | -1.65 |

[a] obtained with the contour deformation implementation in Ref. 2

## III. CP2K INPUT FILE FOR A *GW*100 CALCULATION

```
&FORCE_EVAL
  METHOD Quickstep
  &DFT
    BASIS_SET_FILE_NAME BASIS_def2_QZVP_RI_ALL
    POTENTIAL_FILE_NAME POTENTIAL
    &MGRID
      CUTOFF 400
      REL_CUTOFF 50
    &END MGRID
    &QS
      METHOD GAPW
    &END QS
    &POISSON
      PERIODIC NONE
      PSOLVER  WAVELET
    &END
    &SCF
      EPS_SCF 1.0E-6
      SCF_GUESS RESTART
      MAX_SCF 200
    &END SCF
    &XC
      &XC_FUNCTIONAL PBE
      &END XC_FUNCTIONAL
      &WF_CORRELATION
        &LOW_SCALING
          EPS_FILTER  1.0E-12
          MEMORY_CUT  1
        &END
        &RI_RPA
          RPA_NUM_QUAD_POINTS  30
          &GW
            CORR_MOS_OCC   1
            CORR_MOS_VIRT  1
            SC_GW0_ITER    1
          &END GW
        &END RI_RPA
      &END
    &END XC
  &END DFT
  &SUBSYS
    &CELL
      ABC 25.0 25.0 25.0
      PERIODIC NONE
    &END CELL
    &TOPOLOGY
      COORD_FILE_NAME  01_He.xyz
      COORD_FILE_FORMAT xyz
      &CENTER_COORDINATES
      &END
    &END TOPOLOGY
    &KIND He
      BASIS_SET def2-QZVP
      RI_AUX_BASIS RI-5Z
      POTENTIAL ALL
    &END KIND
  &END SUBSYS
&END FORCE_EVAL
&GLOBAL
  RUN_TYPE     ENERGY
  PROJECT      ALL_ELEC
  PRINT_LEVEL  MEDIUM
&END GLOBAL
```

## IV. GEOMTRY OF THE 24-ATOM PHOSPHORENE SHEET

```
24

P         9.90962        6.97934        4.18948
P         4.80246        4.89076        6.02027
P         4.92455        9.40019        6.24996
P         4.91388        8.47653        4.22120
P        10.01367        5.97752        6.17597
P         5.08646        4.05436        3.99281
P         6.56061        2.50542        4.50140
P         6.61579        7.03377        4.15749
P         8.21070        4.67509        6.24659
P         6.72169       10.66318        6.02716
P         8.20230        9.07741        6.37911
P         8.26869        8.48543        4.26123
P         6.59088        6.19877        6.20542
P         8.34361        3.76985        4.22998
H         6.72736       11.09419        7.41516
H         9.36070        9.95024        6.32325
H         5.42587        8.37214        7.12169
H         3.90585        7.47410        4.51275
H        10.95995        7.93574        4.48953
H         9.62852        6.98804        7.12675
H         5.27874        3.77926        6.82562
H         7.81732        4.78441        3.35459
H         6.57497        1.97849        3.14832
H         3.96581        3.13575        4.08891
```

## V. RI BASIS SET USED FOR APPLYING *GW* TO PHOSPHORENE NANOSHEETS

```
H aug-cc-pVDZ-RIFIT-mod
    9
1 0 0 1 1
      5.11588952             1.0000000
1 0 0 1 1
      1.14296528             1.0000000
1 0 0 1 1
      0.29166153             1.0000000
1 0 0 1 1
      0.15                   1.0000000
1 1 1 1 1
      1.91496403             1.0000000
1 1 1 1 1
      0.98640124             1.0000000
1 1 1 1 1
      0.28586021512          1.0000000
1 2 2 1 1
      1.17208347             1.0000000
1 2 2 1 1
      0.30382076276          1.0000000

P aug-cc-pVDZ-RIFIT-mod
    28
1 0 0 1 1
    228.63267785             1.0000000
1 0 0 1 1
     54.506057893            1.0000000
1 0 0 1 1
     15.762252958            1.0000000
1 0 0 1 1
      7.5544221607           1.0000000
1 0 0 1 1
      3.6842930301           1.0000000
1 0 0 1 1
      1.0949031685           1.0000000
1 0 0 1 1
      0.67469715351          1.0000000
1 0 0 1 1
      0.34651912955          1.0000000
1 0 0 1 1
      0.22114680678          1.0000000
1 0 0 1 1
      0.15                   1.0000000
1 1 1 1 1
    100.33075294             1.0000000
1 1 1 1 1
     15.254506996            1.0000000
1 1 1 1 1
      6.5403548222           1.0000000
1 1 1 1 1
      2.5835737300           1.0000000
1 1 1 1 1
      1.1093869645           1.0000000
1 1 1 1 1
      0.56990264499          1.0000000
1 1 1 1 1
      0.26882922177          1.0000000
1 1 1 1 1
      0.17083085601          1.0000000
1 2 2 1 1
     23.088072722            1.0000000
1 2 2 1 1
      5.5651868450           1.0000000
1 2 2 1 1
      2.8020823738           1.0000000
1 2 2 1 1
      0.63499496425          1.0000000
1 2 2 1 1
      0.38880689308          1.0000000
1 2 2 1 1
      0.2                    1.0000000
1 3 3 1 1
      7.5116747966           1.0000000
1 3 3 1 1
      3.0543024504           1.0000000
1 3 3 1 1
      0.63129177803          1.0000000
1 3 3 1 1
      0.25573460411          1.0000000
```

## VI. INPUT FOR A LARGE-SCALE LOW-SCALING *GW* CALCULATION

```
&FORCE_EVAL
  METHOD Quickstep
  &DFT
    BASIS_SET_FILE_NAME BASIS_H_P
    POTENTIAL_FILE_NAME ALL_POTENTIALS
    SORT_BASIS          EXP
    &MGRID
      CUTOFF 400
      REL_CUTOFF 50
    &END MGRID
    &QS
      METHOD GAPW
      EPS_PGF_ORB           1.0E-80
      EPS_FILTER_MATRIX     1.0E-80
    &END QS
    &POISSON
      PERIODIC NONE
      PSOLVER MT
    &END
    &SCF
      EPS_SCF 1.0E-6
      MAX_SCF 200
    &END SCF
    &XC
      &XC_FUNCTIONAL PBE
      &END XC_FUNCTIONAL
      &WF_CORRELATION
        &LOW_SCALING
          EPS_FILTER 1.0E-15
          MEMORY_CUT 12
        &END
        &RI_RPA
          RPA_NUM_QUAD_POINTS  14
          &GW
            CORR_MOS_OCC   80
            CORR_MOS_VIRT  80
            SC_GW0_ITER    10
          &END GW
        &END RI_RPA
      &END
    &END XC
  &END DFT
  &SUBSYS
    &CELL
      ABC      79.3 106.0 12.0
      PERIODIC NONE
    &END CELL
    &TOPOLOGY
      COORD_FILE_NAME   P.xyz
      COORD_FILE_FORMAT xyz
      &CENTER_COORDINATES
      &END
    &END TOPOLOGY
    &KIND H
      BASIS_SET         aug-cc-pVDZ
      BASIS_SET RI_AUX  aug-cc-pVDZ-RIFIT-mod
      POTENTIAL ALL
    &END KIND
    &KIND P
      BASIS_SET         aug-cc-pVDZ
      BASIS_SET RI_AUX  aug-cc-pVDZ-RIFIT-mod
      POTENTIAL ALL
    &END KIND
  &END SUBSYS
&END FORCE_EVAL
&GLOBAL
  RUN_TYPE     ENERGY
  PROJECT      phosphorene
```

```
  PRINT_LEVEL  MEDIUM
  EXTENDED_FFT_LENGTHS
&END GLOBAL
```

We have used the following parameter to split the spatial part of soft and hard density in the Gaussian and augmented plane waves scheme[3] (GAPW):

```
#
H ALLELECTRON ALL
    1    0    0
     0.20000000    0
#
P ALLELECTRON ALL
    6    9    0
     0.3000000    0
#
```

## VII. RAW DATA OF CALCULATIONS ON THE PHOSPHORENE NANOSHEETS

TABLE III. All HOMO-LUMO gaps in eV. All *GW* calculations in CP2K employ the low-scaling implementation as described in the manuscript. Abbreviations: a-DZ: aug-cc-pVDZ, a-TZ: aug-cc-pVTZ, a-QZ: aug-cc-pVQZ, a-DZ-m: aug-cc-pVDZ using the modified RI basis set from Sec. V and a minimax grid with 14 points. The "tier" indicate the NAO basis sets available in the FHI-aims species library. Note that "tier1+" corresponds to the "really tight" settings in the FHI-aims species definition.

| $L$ | FHI-aims PBE gap | | | | | CP2K PBE gap | | | FHI-aims $G_0W_0$@PBE gap | CP2K ($O(N^3)$ code) $G_0W_0$@PBE gap | | | | CP2K ev$GW_0$@PBE gap |
|---|---|---|---|---|---|---|---|---|---|---|---|---|---|---|
| | a-DZ | tier1 | tier1+ | tier2 | tier3 | a-DZ | a-TZ | a-QZ | a-DZ | a-DZ | a-TZ | a-QZ | a-DZ-m | a-DZ-m |
| 4 | 1.589 | 1.553 | 1.551 | 1.547 | 1.545 | 1.589 | 1.557 | 1.546 | 3.680 | 3.664 | 3.648 | 3.640 | 3.645 | 3.949 |
| 5 | 1.397 | 1.362 | 1.361 | 1.357 | 1.355 | 1.396 | 1.365 | 1.355 | 3.246 | 3.233 | 3.214 | 3.203 | 3.211 | 3.497 |
| 6 | 1.278 | 1.244 | 1.244 | 1.240 | 1.238 | 1.277 | 1.247 | 1.237 | 2.961 | 2.944 | | | 2.929 | 3.202 |
| 8 | 1.131 | 1.099 | 1.098 | 1.095 | 1.093 | 1.130 | 1.100 | 1.091 | | | | | 2.573 | 2.828 |
| 10 | 1.052 | 1.020 | 1.020 | 1.017 | 1.015 | 1.053 | 1.024 | 1.015 | | | | | 2.378 | 2.620 |
| 12 | 1.001 | 0.968 | 0.967 | 0.965 | | 1.001 | 0.973 | 0.963 | | | | | 2.253 | 2.488 |
| 15 | 0.949 | 0.916 | 0.916 | | | 0.949 | 0.920 | 0.911 | | | | | 2.130 | 2.357 |
| 20 | | 0.868 | | | | 0.901 | 0.872 | 0.862 | | | | | | |

* jan.wilhelm@physik.uni-regensburg.de
1 M. J. van Setten, F. Caruso, S. Sharifzadeh, X. Ren, M. Scheffler, F. Liu, J. Lischner, L. Lin, J. R. Deslippe, S. G. Louie, C. Yang, F. Weigend, J. B. Neaton, F. Evers, and P. Rinke, *J. Chem. Theory Comput.* **2015**, *11*, 5665–5687.
2 D. Golze, J. Wilhelm, M. J. van Setten, and P. Rinke, *J. Chem. Theory Comput.* **2018**, *14*, 4856–4869.
3 G. Lippert, J. Hutter, and M. Parrinello, *Theor. Chem. Acc.* **1999**, *103*, 124–140.
